# Supplementary material for: Further investigation of dilepton-based center-of-mass energy measurements at e$^{+}$e$^{-}$ colliders
Source: arXiv:2308.10414 source file (2023-08-21)
Supplement: Supplementary file 1 [file Appendix.tex]

\newpage
\appendix

\section{Example WHIZARD Sindarin File}\label{sec:A1}
\begin{minted}[linenos,fontsize=\footnotesize]{vhdl}
model = SM_Higgs_CKM
mmu = 0.105658
me = 0.000511
mW = 80.419
mZ = 91.1876

polarized "e1","E1","e2","E2"

sample_format = lhef

process mumu = "e1", "E1" => ("e2","E2") + 
    ("e2", "E2", "A") + ("e2", "E2", "A", "A") + 
    ("e2", "E2", "A", "A", "A")

cuts = all 5 degree < Theta < 175 degree [e2] and
    all 5 degree < Theta < 175 degree [E2]

beams = e1, E1 => isr, isr
#beams_momentum = 0.5 * VCOM , 0.5 * VCOM
#beams_theta = 0.802 degree , 0.802 degree
#!isr_order         = 3
?isr_handler       = true
$isr_handler_mode  = "recoil"
isr_alpha          = 0.0072993
isr_mass           = 0.000511
beams_pol_density = @(+1), @(-1)
beams_pol_fraction = 80%, 30%

n_events = VNEV

compile

sqrts = VCOM
integrate (mumu) { iterations = 20:10000 }

simulate (mumu)

write_analysis
compile_analysis { $out_file = "mumu.dat" }
\end{minted}
